# Supplementary material for: Lucid: A Language for Control in the Data Plane
Source: arXiv:2107.02244 source file (2021-07-05)
Supplement: Supplementary file 1 [file appendixcompiler.tex]

\section{Single-operation P4 Tables}
\label{app:backendfirstpass}
The back-end of \lang's compiler translates primitive \lang statements generated by the front end into \emph{single-operation P4 tables}. There are three types of primitive \lang statements, that each use a different template to translate into a P4 table. 

\subheading{Binary operations} A binary operation evaluate a binary expression over local variables and assign its result to a (possibly new) local variable. The compiler translates a binary operation into a P4 action wrapped with a and table. For example, \inl{idx = idx + NUM_PORTS;} translates to: 
\begin{lstlisting}[style=P4Snip]
action do_idx_eq_0 {idx = idx + NUM_PORTS;}
table idx_eq_0 {	
	actions = {do_idx_eq_0;}
	const default_action = {do_idx_eq_0;}
}
\end{lstlisting}

\subheading{Stateful operations} A Stateful operation is a call to 
a data structure method that operates on a global variable. The compiler translates this call to a table that executes a co-generated \inl{RegisterAction}. The body of the \inl{RegisterAction} is a direct (but verbose) translation of the \inl{memops} passed in the call. For example, here is the register action generated by the call \inl{Array.fset(tcp_cts, port, plus, 1);}.
\begin{lstlisting}[style=P4Snip]
RegisterAction<bit<32>,bit<32>,bit<32>>
  (tcp_cts) fset_1 = {
  void apply(inout bit<32> mem, out bit<32> ret) {
    mem = mem + 1;
  } };
\end{lstlisting}
The translation from \inl{memop} to \inl{RegisterAction} can be direct because the syntactic restrictions of \inl{memops} guarantees that they can compile to the Tofino's stateful ALUs.

\subheading{Branch operations} A branch operation is an \inl{if}/\inl{else} statement that evaluates a simplified conditional expression. The simplified expression is a conjunction or disjunction of clauses that each compare a local variable with a constant. A branch operation translates to a table that evaluates the conditional expression using ternary rules and calls a true or false action. For example, \inl{if(proto != TCP)} translates to:
\begin{lstlisting}[style=P4Snip]
action if_0_true(); action if_0_false();
table if_0 {	
	keys = {proto : ternary;}
	actions = {if_0_true; if_0_false;}
	entries = {
		(TCP) : if_0_false;
		(_)   : if_0_true;
}	}
\end{lstlisting}
The compiler also generates a table of this form to select between handlers based on an event ID field.
