# Supplementary material for: Lucid: A Language for Control in the Data Plane
Source: arXiv:2107.02244 source file (2021-07-05)
Supplement: Supplementary file 2 [file appendixexample.tex]

\cleardoublepage
\let\clearpage\relax
\section{The \exprog in \lang}

\begin{figure}[t]
	\begin{lstlisting}[style=DptBlock,xleftmargin=1.5ex,xrightmargin=.5ex]
	// An IP packet enters or exits the program.
	packet entry event !ip_in!(int<32> dst);
	packet exit event !ip_out!(int<8> egrPort);
	// A request to ensure that the route at idx is valid.
	support event !do_check_route!(int<32> idx);
	// A query from switch s for the path length to dst.
	support event !pLenQ!(int<32> s, int<32> dst);
	// An answer from switch s with its path length to dst.
	support event !pLenA!(int<32> s, int<32> dst, int<8> len);
	// A request to ping all neighboring switches.
	support event !do_ping!(int<32> pingId);
	// A ping from neighbor switch s.
	support event !pingQ!(int<32> s, int<32> pingId);
	// A ping response from neighbor switch s.
	support event !pingA!(int<32> s, int<32> pingId);
	\end{lstlisting}
	\caption{Event declarations in the \exprog.}
	\vspace{2em}
	\label{fig:eventdecls}
\end{figure}

\begin{figure}[t]
    \begin{lstlisting}[style=DptBlock]
const int NO_ROUTE = Sys.MAX_32;
const int T_DOWN = 10000; // 10ms

// events
packet entry event ip_in(int dst);
packet exit  event ip_out(int port);

// state 
// map dst --> (shortest known pathlen, next hop)
global nexthop_pathlen 	= new Array<<32>>(tbl_sz);
global nexthop_nid 	= new Array<<32>>(tbl_sz);

// map neighbor --> (last pinged time, port)
global last_seen = new Array<<32>>(neighbor_ct);
global nid_port = new Array<<32>>(neighbor_ct);

// routing failure counter
global noroute_ct = new Array<<32>>(tbl_sz);

// memops
// check if stored timestamp is older than T_DOWN
memop threshold_exceeded(int stored_ts, int cur_ts) {
	if (cur_ts - stored_ts > T_DOWN) {
		return TRUE;
	}
	else {
		return FALSE;
	}
}
// increment the stored value.
memop incr(int stored_val, int incr_by) {
	return stored_val + incr_by;
}

// Get a next hop, if it is still valid. 
fun int get_outport(int dst) {
	int ts = Sys.time();	
	int next_hop = Array.get(nexthop_nid, dst);
	int nexthop_is_down = Array.getm(last_seen, next_hop, nid_is_down, ts);
	if (next_hop != NO_ROUTE && nexthop_is_down == FALSE) {
		int outport = Array.get(nid_port, next_hop);
		return outport;
	}
	else {
		return NO_ROUTE;
	}
}

// Log a routing failure. 
fun void log_failure(int dst) {
	Array.setm(noroute_ct, dst, incr, 1);
}

// Handle an IP packet by looking up its output port
// if none is found, increment a failure counter.
handle ip_in(int dst) {
	int outport = get_outport(dst);
	if (next_hop != NO_ROUTE) {
		generate ip_out(outport);
	}
	else {
		log_failure(dst);
	}
}
    \end{lstlisting}
    \caption{Forwarding component of the \exprog in \lang.}
    \label{fig:exhandlers}
\end{figure}

\begin{figure}[t]
    \begin{lstlisting}[style=DptBlock]
const int INF = Sys.MAX_32;
const int T_PAUSE = 1000 // 1ms

// check to see if route i is valid. 
support event check_route(int i);
// query to/reply from a neighbor for path length. 
support event qry_pathlen(int srcid, int dst);
support event rep_pathlen(int srcid, int dst, int pathlen);

fun void query_neighbors(int dst) {
	mgenerate Event.smlocate(qry_pathlen(SELF, i), NEIGHBORS);
}
handle check_route(int i) {
	int ts = Sys.time();
	int pathlen = Array.get(nexthop_pathlen, i);
	if (pathlen == INF) {
    	query_neighbors(i);
	}
	else {
		int outport = get_outport(i);
		if (outport == NO_ROUTE) {
        	query_neighbors(i);
		}
	}
	// scan the next entry in the routing table. 
	int next_i = i + 1;
	if (next_i == TBL_SZ) {
		generate Event.delay(check_route(0), T_PAUSE);
	}
	else {
		generate check_route(next_i);
	}
}
handle query_pathlen(int src_id, int dst) {
	int pathlen = Array.get(nexthop_pathlen, dst);
	generate Event.sslocate(reply_pathlen(SELF, dst, pathlen), src_id);
}
memop comp_pathlen(int cur_pathlen, int neighbor_pathlen) {
	if (neighbor_pathlen + 1 < cur_pathlen) {
		return TRUE;
	}
	else {
		return FALSE;
	}
}
memop upd_pathlen(int cur_pathlen, int neighbor_pathlen) {
	if (neighbor_pathlen + 1 < cur_pathlen)  {
		return neighbor_pathlen + 1;
	}
	else{
		return cur_pathlen;
	}
}
// If src has a shorter path to dst, update nexthop.
handle reply_pathlen(int src, int dst, int pathlen){
	int found_shorter = Array.update(nexthop_pathlen, dst, test_path_change, pathlen, update_pathlen, pathlen);
	if (found_shorter == TRUE) {
		Array.set(nexthop_nid, dst, src);
	}
}
    \end{lstlisting}
    \caption{Routing component of the \exprog in \lang.}
    \label{fig:exhandlers}
\end{figure}
