# Supplementary material for: Lucid: A Language for Control in the Data Plane
Source: arXiv:2107.02244 source file (2021-07-05)
Supplement: Supplementary file 3 [file appendixgrammar.tex]

\section{\lang Grammar}
\label{app:grammar}

\begin{figure}[H]
\makeunderscoreactive
\footnotesize
\noindent\rule{\columnwidth}{.1em}
\raggedright {\textbf{declarations}}
\setlength{\grammarindent}{1em}
\begin{grammar}
<decl> ::=\lit{const} <type> <const_var_id> \lit{=} <value> \lit{;} 	\hfill (constant variable)
\alt `global'<var_id>`=new'<module_id>`<'<size>`>('<args>`);'	\hfill(global obj.)
\alt <event_qualifier> `event' <event_id> `('<params>`);'	\hfill (event)
\alt `handle' <event_id> `('<params>`)' `{'<stmt>`}'		\hfill (handler)
\alt `fun' <type> <function_id> `('<params>`)' `{'<stmt>`}'		\hfill (function)
\alt <memop_decl>                   \hfill (function operating on persistent state)
% \alt `memop' <callable_id> `('<params>`)' `{'<stmt>`}'		\hfill (memory op.)
\end{grammar}
{\raggedright \textbf{statements}}
\begin{grammar}
<stmt> ::= <no_op>											
\alt <stmt> `;' <stmt> 										\hfill (sequence)
\alt `if(' <expr> '){'<stmt>'}'[`else {'<stmt>`}'] 			\hfill (branch)
\alt <type> <var_id> [`=' <expr> ]`;' 						\hfill (local variable declaration)
\alt <var_id> `=' <expr> `;'								\hfill (local variable assignment)
\alt <expr> `;'												\hfill (call to function and ignore return)
% \alt <callable_id> `('<args>`)' `;'							\hfill (call to function with no return)
% Technically, a procedure call has the syntax <expr>; -- but maybe it is clearer if we write it out?
\alt `generate' <expr> `;'									\hfill (generate event)
\alt `return' <expr> `;' 									\hfill (return from inside of function)
% omitted: print statements -jsonch
\end{grammar}
{\raggedright \textbf{expressions}}
\begin{grammar}
<expr> ::= <value> | <var_id> 								
\alt <expr> <bin_op> <expr>									\hfill (binary operation)
\alt <callable_id> `('<args>`)'								\hfill (function call)
\alt `hash<'<size>`>('<args>`)' 							\hfill (hash operation)
% omitted line for: "| EInt of z * size option" -- unsure of purpose and how to describe. -jsonch
\end{grammar}
{\raggedright \textbf{miscellaneous}}
\setlength{\grammarindent}{0em}
\begin{grammar}
<value> ::= <bool> | <int>[`<'<size>`>']					\hfill (values) \\
<bin_op> ::= `+' | `-' | `|' | `&' | `==' | `>' | `<' | ... \hfill (operations) \\
<params> ::= [<type> <var_id> [`,' <type> <var_id>]*] 		\hfill (parameters) \\
<args> ::= [<expr> [,<expr>]*]								\hfill (arguments) \\
<type> ::= `int<' <size> `>' | `bool' | `void' | `auto' 	\hfill (types) \\
<size> ::= <const_var_id> | <int> 							\hfill (variable sizes)\\
<callable_id> ::= <function_id> | <module_id>\lit{.}<builtin_id> \hfill (subroutines)
% type grammar is probably not right. Unsure of which nodes in the type syntax tree correspond to written code. There are also type variables, for example... -jsonch
\end{grammar}
% \vspace{-0.5em}
\noindent\rule{\columnwidth}{.1em}%
\caption{The \lang language grammar.}
\vspace{4pt}
\label{fig:gram}
\makeunderscoreletter
\end{figure}

\begin{figure}[H]
% \makeunderscoreactive
\footnotesize
\noindent\rule{\columnwidth}{.1em}
\raggedright{\textbf{\code{memop} declarations.}}
\setlength{\grammarindent}{0em}
\begin{grammar}
<memop_decl> ::= `memop' <callable_id> `('<m_params>`)' `{'<m_stmt>`}'\\
<m_params> ::= <type> <var_id> `,' <type> <var_id>\\
<m_stmt> ::= <ret_stmt> \\ 
"\quad"| `if (' <test_exp> `){' <ret_stmt> `}' [`else {'<ret_stmt> `}']
\end{grammar}
\raggedright{\textbf{\code{memop} return statements.}}
\begin{grammar}
<ret_stmt> ::= `return' <ret_exp> `;'\\
<ret_exp> ::= <simple_exp> | <simple_exp> <op> <simple_exp>\\
<op> ::=  `+' | `-' | `&' | `|' | `^'\\
<simple_exp> ::= <const> | <m_param>
\end{grammar}
\raggedright{\textbf{\code{memop} if/else statements.}}
\begin{grammar}
<test_exp> ::= <math_exp> <cmp_op> <math_exp>\\
<math_exp> ::= <simple_exp> <math_op> <simple_exp>\\
<math_op> ::= `+' | `-'\\
<cmp_op> ::= `>' | `<' | `==' | `!=' | `>=' | `<='
\end{grammar}
\vspace{-0.5em}
\noindent\rule{\columnwidth}{.1em}
\caption{The restricted grammar of memory operations. Each \code{memop} parameter (\synt{m_param}) may only appear once in a \synt{ret_exp} and \synt{test_exp}.}
\label{fig:memopgram}
\vspace{4pt}
% \makeunderscoreletter
\end{figure}

Figure~\ref{fig:gram} lists the grammar of \lang, 
while Figure~\ref{fig:memopgram} lists the grammar of \lang's syntactically restricted memory operations.
